# Supplementary material for: ReMoDiffuse: Retrieval-Augmented Motion Diffusion Model
Source: arXiv:2304.01116 source file (2023-04-03)
Supplement: Supplementary file 1 [file supp_03_pose.tex]

\section{Exploration on Pose Retrieval}

Inspired by AvatarCLIP~\cite{hong2022avatarclip}, we aim to retrieve a relevant pose based on the user input and use these retrieved poses to enhance the motion generation results. The following subsections briefly introduce the pose retrieval technique used in the AvatarCLIP. Then we will illustrate how to incorporate these candidate poses into the motion generation pipeline.

\subsection{Pose Retrieval}

As shown in Figure ~\ref{fig:pipeline_clip}, we get poses from the amass dataset to form a large-scale codebook containing millions of pose data. To better reduce the size, we first use VPoser to encode each pose into a 32-d dimensionality and use K-means clustering to get 1024 cluster centroids. For each cluster centroid, we acquired the original pose parameter by using the VPoser decoder. Rendered from different views, we get a series of pictures of a single 3D gesture. CLIP~\cite{radford2021learning} is applied here to get visual features. During the training period and inference time, we retrieve $k$-th most similar poses from the database by calculating the similarity between the text and visual features. These poses will be sent to the cross-attention module to enhance the motion generation process.

\begin{figure}[t]
    \centering
    \includegraphics[width=\linewidth]{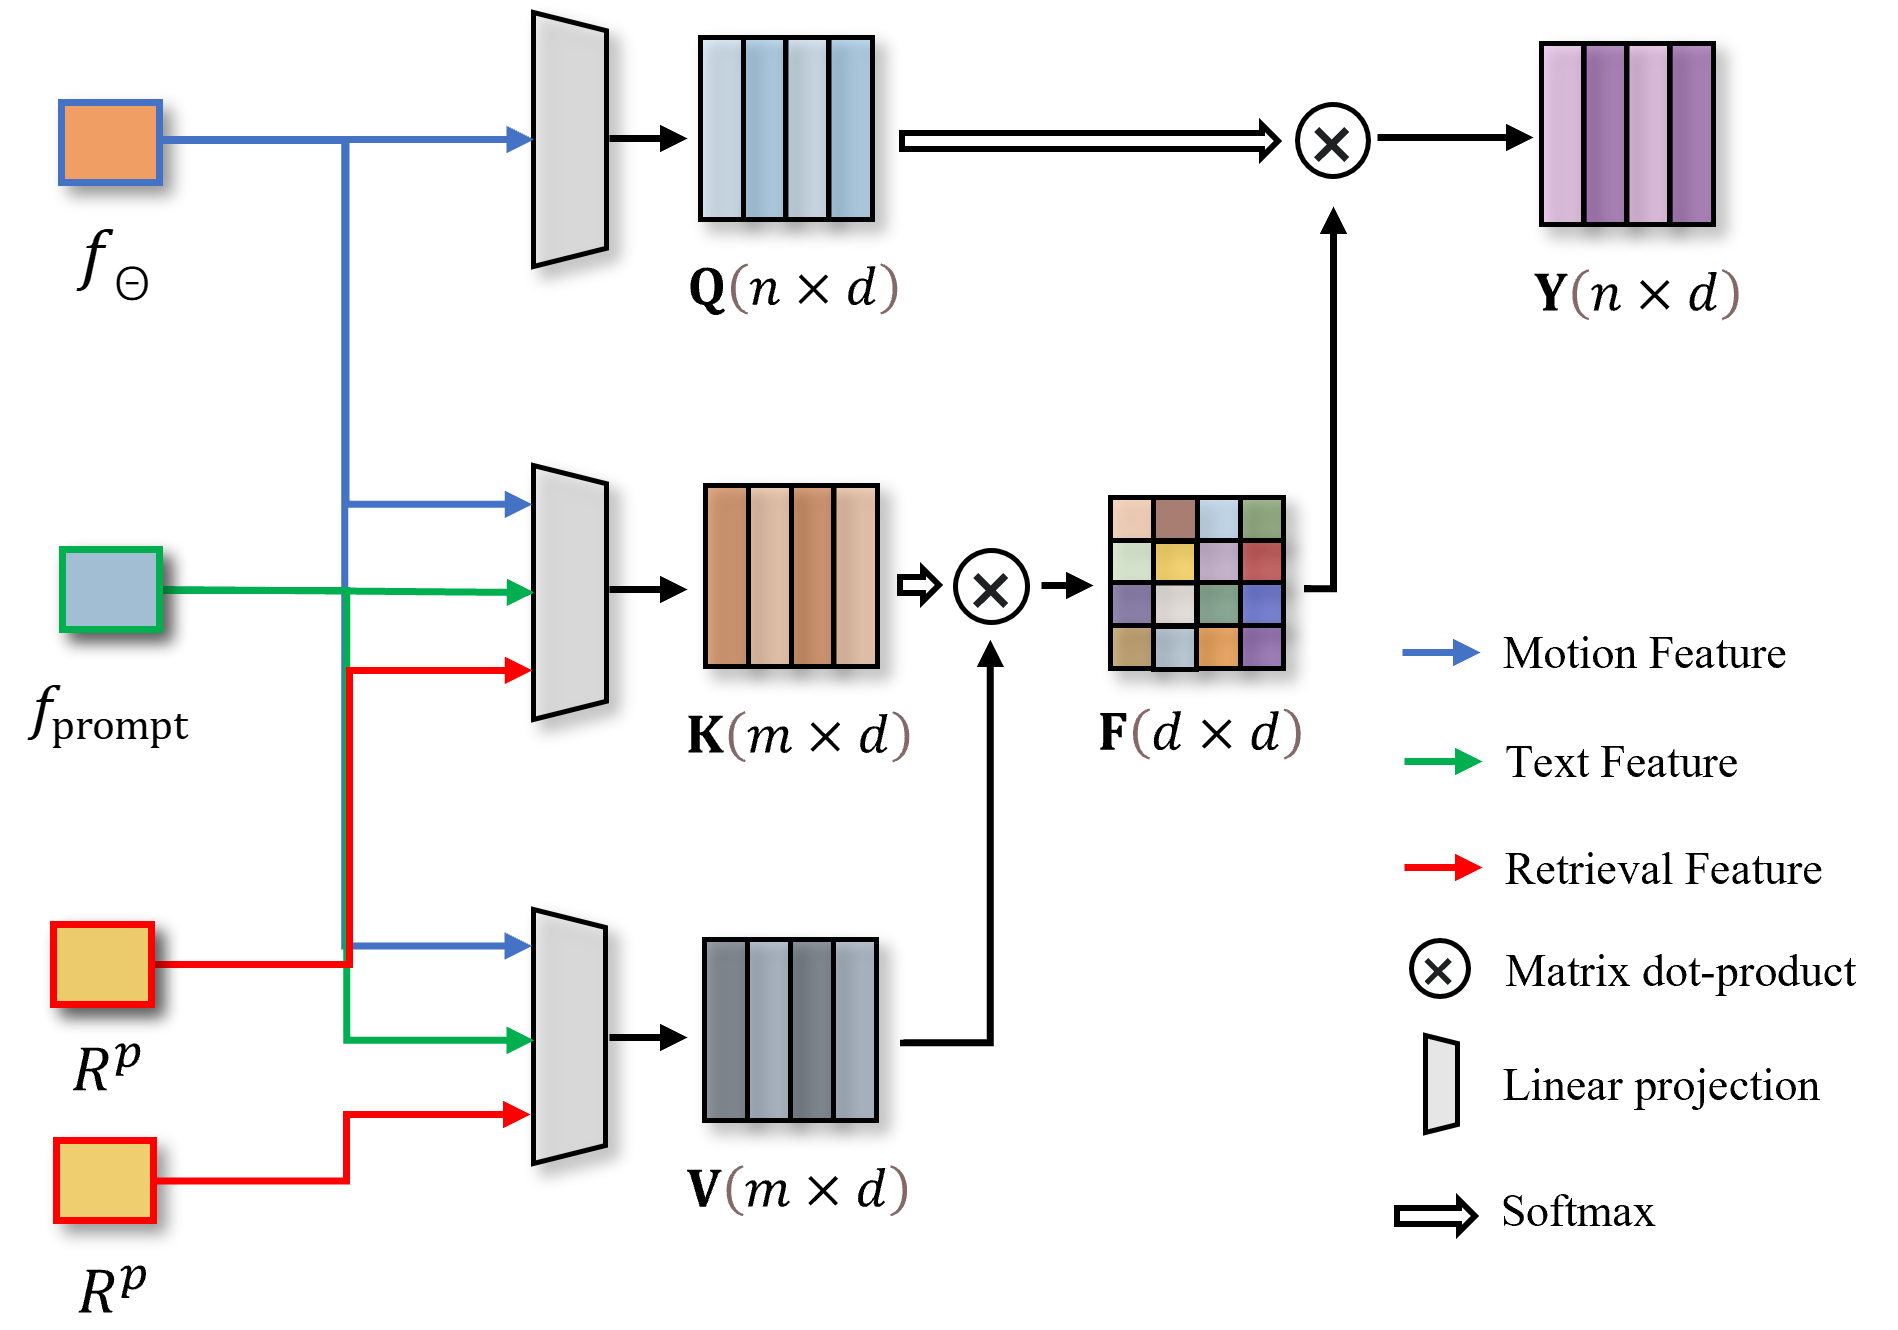}
    \caption{\textbf{The structure of Modified Semantic-Modulated Attention.}}
    \label{fig:modified_attention}
\end{figure}

\begin{figure}[t]
    \centering
    \includegraphics[width=\linewidth]{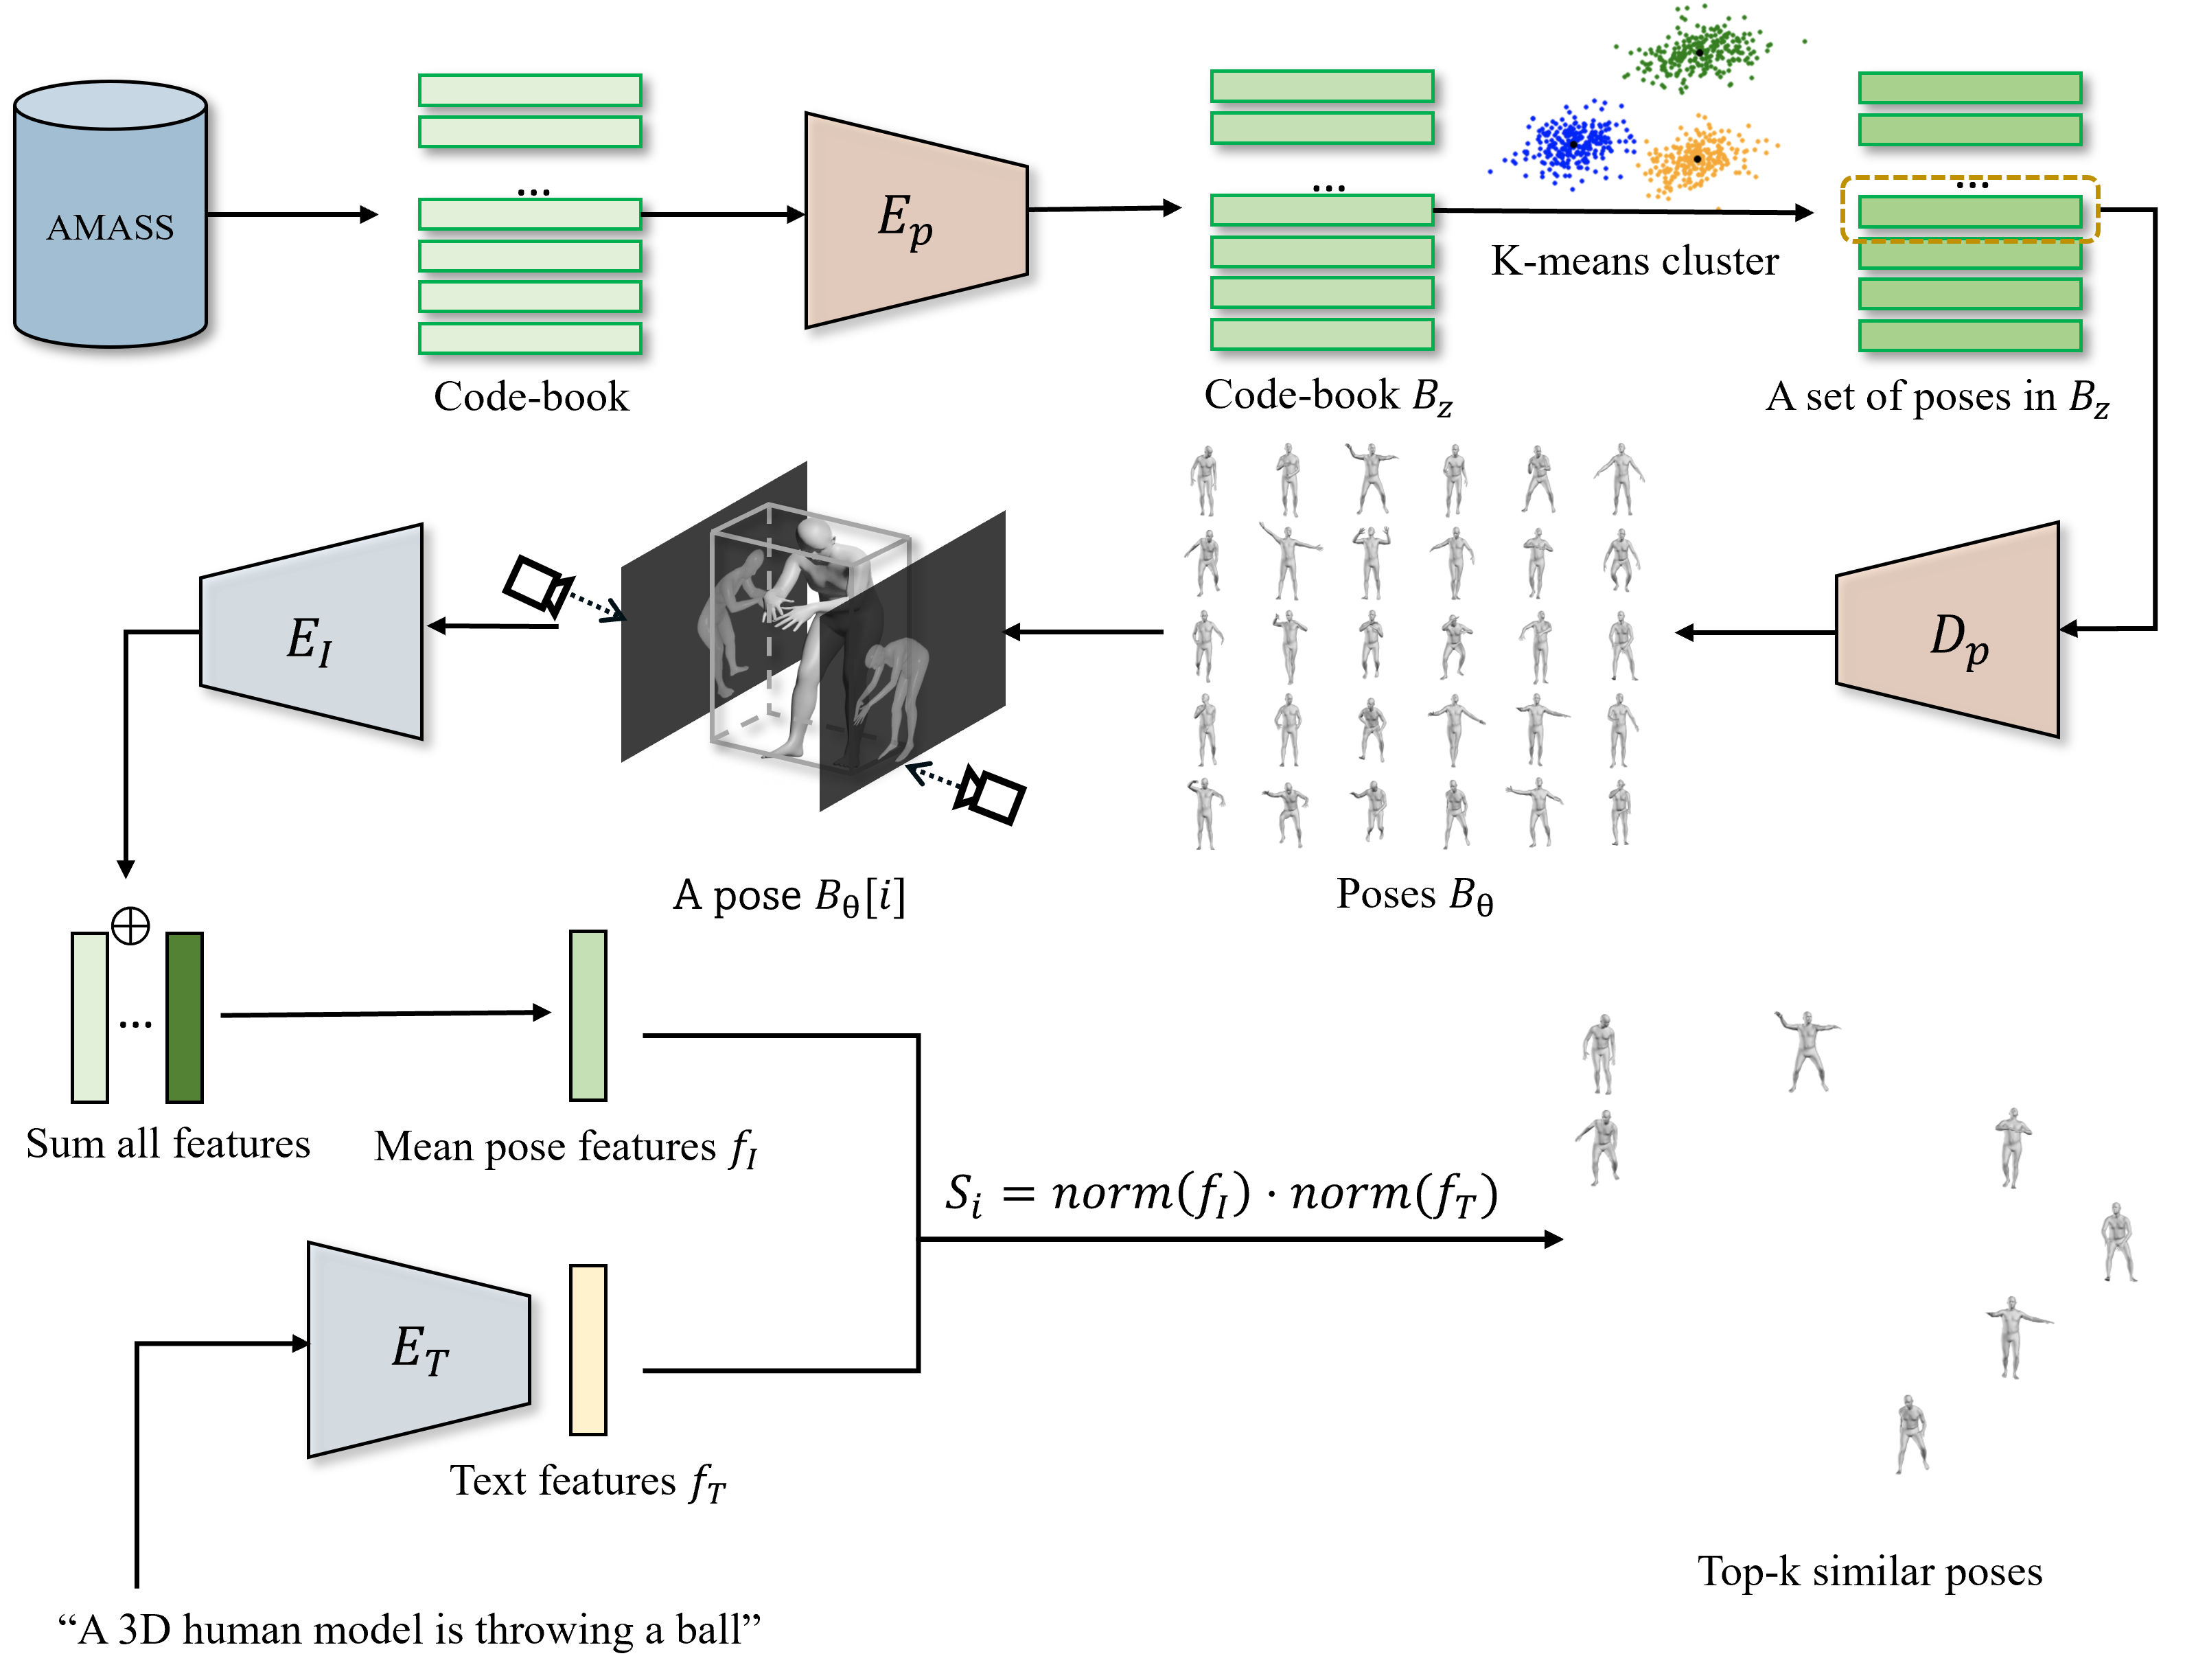}
    \caption{\textbf{Pose Retrieval Pipeline in AvatarCLIP~\cite{hong2022avatarclip}}}
    \label{fig:pipeline_clip}
\end{figure}

\begin{figure*}[t]
    \centering
    \includegraphics[width=\linewidth]{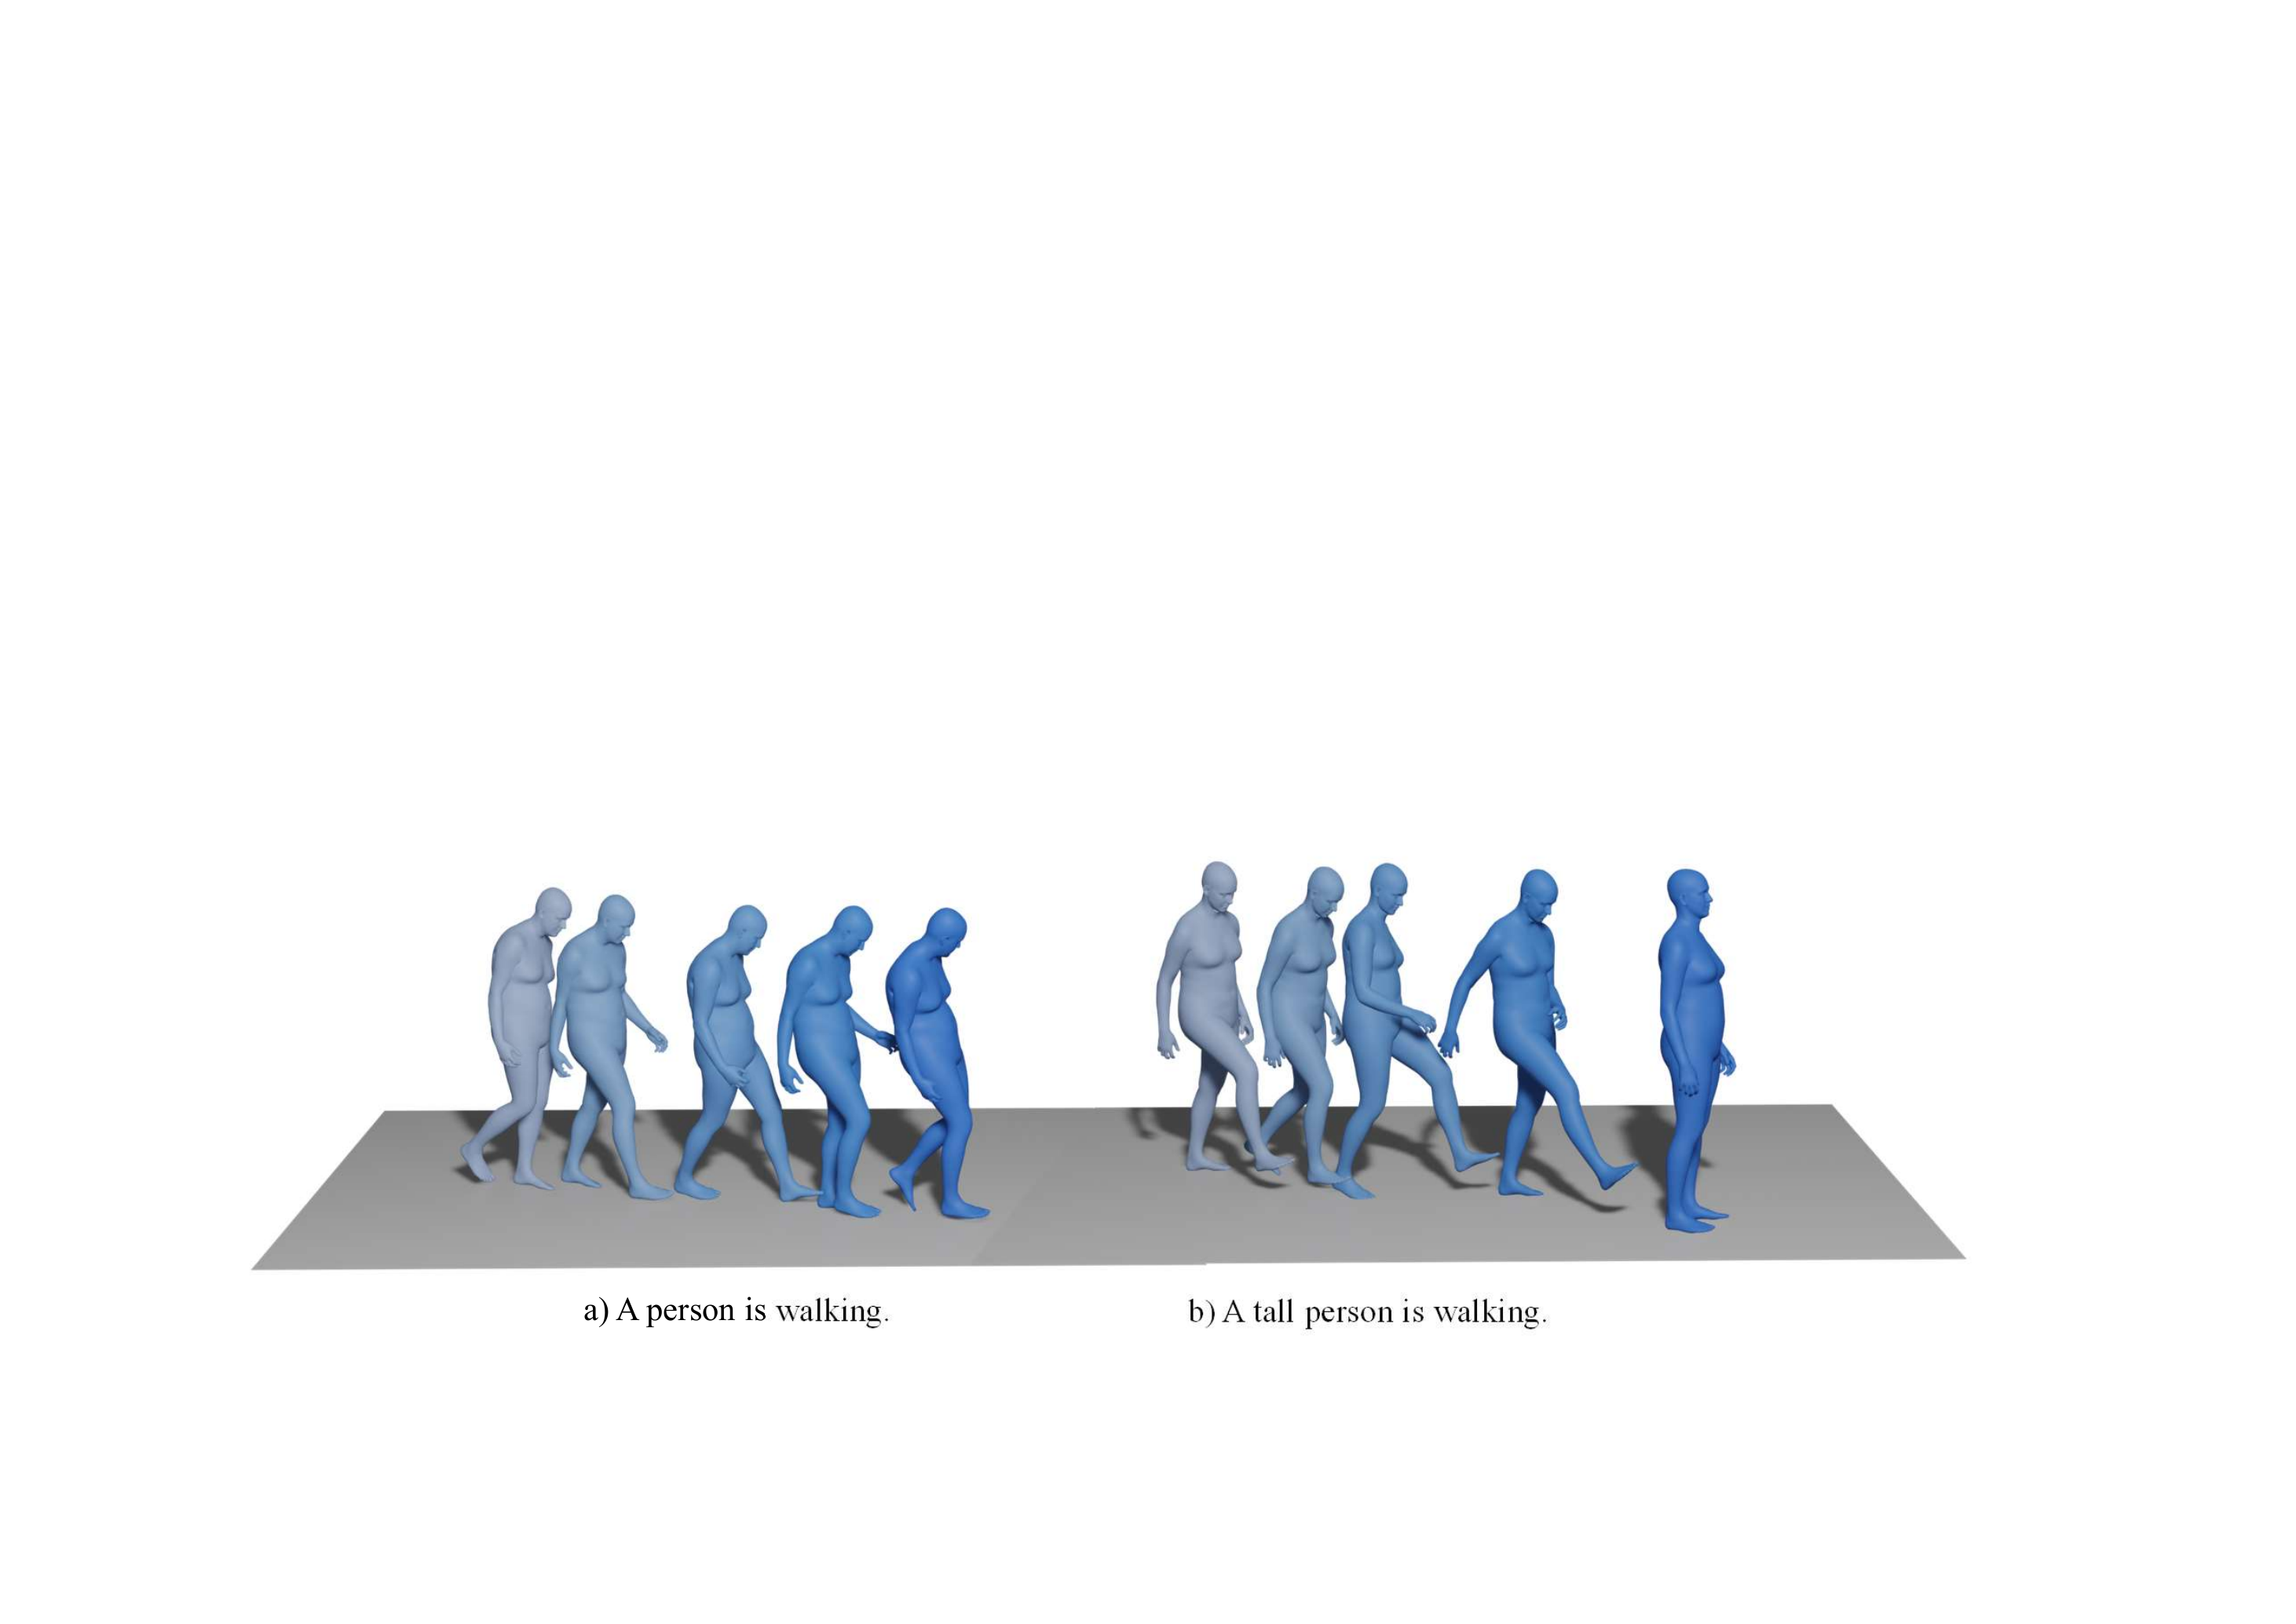}
    \caption{\textbf{Visualization of Pose-enhanced \name}}
    \label{fig:vis_pose}
\end{figure*}

\subsection{Modified Semantics-Modulated Attention}

Unlike retrieved motion sequences, here we select the top 2 poses and embed the pose parameters into feature vectors. These vectors are directly used to refine motion sequences as shown in Figure ~\ref{fig:modified_attention}. Other settings remain unchanged.

\subsection{Experimental Results}

\begin{table}[t]
\centering
\caption{\textbf{Quantitative results of pose retrieval on KIT testset.}}
\label{tab:pose}
\setlength{\tabcolsep}{1.4mm}
{
\begin{tabular}{ccc}
\hline

Method & Top 1$\uparrow$ & FID$\downarrow$ \\
\hline
Baseline & $0.421^{\pm.012}$ & $0.245^{\pm.008}$ \\
Pose Retrieval & $0.422^{\pm.012}$ & $0.251^{\pm.009}$ \\
\hline
\end{tabular}}
\vspace{-10pt}
\end{table}

This section provides some preliminary evaluation of the pose retrieval technique. As shown in Table ~\ref{tab:pose}, the quantitative results are almost the same when we use selected poses to enhance the motion generation process. However, we find some other interesting uses of this technique. Figure ~\ref{fig:vis_pose} shows the generated motion sequences with two different given text descriptions. The only difference between them is that we describe the body shape in the second one. It should be mentioned that, in the KIT-ML dataset, we use 3D key points as the primary motion representation. The visualized meshes are generated from SMPLify~\cite{bogo2016keep}. The visual feature of our retrieved poses may be consistent with the description "tall", thereby guiding the denoising steps to synthesize a motion sequence with a tall skeleton. 

This technique may be further explored and can be a significant supplementary to our \name, enhancing the consistency between visual description and the synthesized motion sequences.
